# Supplementary material for: Label-efficient Hybrid-supervised Learning for Medical Image Segmentation
Source: arXiv:2203.05956 source file (2022-03-10)
Supplement: Supplementary file 1 [file appendix.tex]

% \maketitle
\clearpage
% \pagenumbering{roman}
% \normalsize
\appendix

\section{Appendix}
% \section{Details for Dynamic Instance Indicator}

\subsection{Details for DII Gradient Estimation}
For the sake of completeness, we present a brief derivation of the DII gradient estimation.
As discussed in the main paper, calculating the gradient of DII involves the differentiating through the lower-level training procedure:
\begin{equation}
\begin{aligned}
    \theta^*(\Gamma) &= \argmin_{\theta} \mathcal{L}(\mathcal{D},\theta,\Gamma ) \\
    % & =\argmin_\theta 
    % \left[
    % \mathcal{L}(\mathcal{D}_S,\theta) + \mathcal{L}(\mathcal{D}_W,\theta,\Gamma)
    % \right] \\
    & =\argmin_\theta 
    \left[
    \mathcal{L}(\mathcal{D}_S,\theta) + \frac{1}{M} \sum_{k=1}^{M} \gamma_k \ell (\mathbf{x}_k, \mathbf{y}_k,\theta)
    \right].
\end{aligned}
\end{equation}
Recall that we decompose the DII gradient w.r.t $\gamma_k$ of $k$-th instance in Eq. 2 of the main paper as:
\begin{equation}
\label{eq:decomposition}
    \frac{\partial \mathcal{L}(\mathcal{D}_S,\theta^*(\Gamma) ) }{ \partial \gamma_k } = \nabla_\theta \mathcal{L} \left(\mathcal{D}_S,\theta^*(\Gamma) \right)^\top \cdot \ \frac{\partial \theta^*(\Gamma)}{\partial \gamma_k} .
\end{equation}
We assume that $\mathcal{L}$ is twice-differentiable and strictly convex in $\theta$ and thus the Hessian 
\begin{equation}
\label{eq:hessian}
H_\theta=\nabla^2 \mathcal{L} (\mathcal{D},\theta^*,\Gamma)
\end{equation}
exists and is positive definite, which also ensures that the Hessian $H_\theta$ is invertible.

The key to the gradient estimation is approximating $\frac{\partial \theta^*(\Gamma)}{\partial \gamma_k} $.
We compute the partial derivative following the derivative definition:
\begin{equation}
\label{eq:derivative_definition}
    \frac{\partial \theta^*}{\partial \gamma_k} 
    = 
    \left.
    \frac{\theta^*_{\epsilon,k} - \theta^*}{\epsilon} 
    \right| _{\epsilon \rightarrow 0} ,
    % =
    % \left.
    % \frac{ \Delta_\epsilon }{ \epsilon }
    % \right| _{\epsilon \rightarrow 0},
    % = 
    % - H^{-1}
    % \ell (\mathbf{x}_k, \mathbf{y}_k, \theta^*)
\end{equation}
where $\epsilon \rightarrow 0$ is a small value that upweighting the $k$-th weakly-annotated instance via $\gamma_k \leftarrow \gamma_k + \epsilon$, and $\theta^*_{\epsilon,k}$ indicates the optimal parameters of lower-level network using new $\gamma_k$. The new parameters can be formulated as:
\begin{equation}
    \theta^*_{\epsilon,k} =
    \argmin_\theta \left[
    \mathcal{L}(\mathcal{D},\theta,\Gamma) + \epsilon \ell (\mathbf{x}_k, \mathbf{y}_k, \theta)
    \right].
\end{equation}
As $\theta^*_{\epsilon,k}$ minimizes the above objective, we examine the first-order optimality conditions:
\begin{equation}
    \nabla_{\theta} \mathcal{L}(\mathcal{D},\theta^*_{\epsilon,k},\Gamma)
    +
    \epsilon \nabla_{\theta} \ell (\mathbf{x}_k, \mathbf{y}_k, \theta^*_{\epsilon,k}) = 0.
\end{equation}
Here, we define the parameter change $\Delta_\epsilon=\theta^*_{\epsilon,k} - \theta^*$.
Since $\epsilon \rightarrow 0$ and $\theta^*_{\epsilon,k} \rightarrow \theta^*$, we can apply Taylor expansion on the left-hand side:
\begin{equation}
\begin{aligned}
    & \left[ 
    \nabla_{\theta} \mathcal{L} \left(\mathcal{D},\theta^* ,\Gamma\right)
    +
    \epsilon \nabla_{\theta} \ell (\mathbf{x}_k, \mathbf{y}_k, \theta^*)
    \right]
    + \\
    & \left[
    \nabla_{\theta}^2 \mathcal{L} \left(\mathcal{D},\theta^* ,\Gamma\right)
    +
    \epsilon \nabla_{\theta}^2 \ell (\mathbf{x}_k, \mathbf{y}_k, \theta^*)
    \right]
    \Delta_\epsilon 
    \approx 0 ,
\end{aligned}
\end{equation}
where we have dropped the higher order terms $o(\| \Delta_\epsilon  \|)$.
Solving for $\Delta_\epsilon$, we have:
\begin{equation}
\begin{aligned}
    \Delta_\epsilon \approx
    & -
    \left[
    \nabla_{\theta}^2 \mathcal{L} \left(\mathcal{D},\theta^* ,\Gamma\right)
    +
    \epsilon \nabla_{\theta}^2 \ell (\mathbf{x}_k, \mathbf{y}_k, \theta^*)
    \right] ^{-1} \\
    & \left[ 
    \nabla_{\theta} \mathcal{L} \left(\mathcal{D},\theta^* ,\Gamma\right)
    +
    \epsilon \nabla_{\theta} \ell (\mathbf{x}_k, \mathbf{y}_k, \theta^*)
    \right] .
\end{aligned}
\end{equation}
Since $\theta^*$ minimize $\mathcal{L}$, we have $\nabla_{\theta} \mathcal{L} \left(\mathcal{D},\theta^* ,\Gamma\right) = 0$.
We further ignore $\epsilon \nabla_{\theta}^2 \ell (\mathbf{x}_k, \mathbf{y}_k, \theta^*)$, and then get:
\begin{equation}
\begin{aligned}
    \Delta_\epsilon \approx
    & -
    \nabla_{\theta}^2 \mathcal{L} \left(\mathcal{D},\theta^* ,\Gamma\right)
    ^{-1} 
    \cdot
    \epsilon \nabla_{\theta} \ell (\mathbf{x}_k, \mathbf{y}_k, \theta^*).
\end{aligned}
\end{equation}
Combining with \Eq\ref{eq:hessian} and \Eq\ref{eq:derivative_definition}, we finally get:
\begin{equation}
    \frac{\partial \theta^*}{\partial \gamma_k} 
    = 
    - H_\theta^{-1}
    \nabla_{\theta} \ell (\mathbf{x}_k, \mathbf{y}_k, \theta^*).
\end{equation}
% 

% \subsection{Details for Per-instance Gradient}
\subsection{Details about DII Optimizer}
Benefiting from efficient approximation and batch parallelism, we can efficiently compute the gradients for all instances.
% It is also worth noting that we update all DIIs $\Gamma$ directly using the vanilla Adam optimizer.
Recall that we are performing gradient descent on $\gamma_k \in \Gamma$ only if the loss $\mathcal{L}$ depends on $(\mathbf{x}_k,\mathbf{y}_k)$.
Meanwhile, we utilize a single vanilla Adam optimizer to maintain all DIIs $\Gamma$.
To avoid incorrect momentum values updated by moving averages, unlike network optimization, which computes gradients w.r.t parameters $\theta$ on each mini-batch and updates $\theta$ in time, the gradient descent step for DIIs $\Gamma$ is performed after computing gradients for all instances in $\mathcal{D}_W$.

% \subsection{Additional Discussion}

\subsection{Additional Visualizations}
\Fig\ref{fig:dii_supp} demonstrates additional training pairs and corresponding DII values.
We observed that 1) DII pushes instances containing irrelevant images, blurred images, and mislabeled images to zero weight; 
2) high-quality instances, \textit{i.e.}, those containing clear polyps and relatively accurate annotations, are pushed toward one weight; and 3) a considerable fraction of the instances fall between 0 and 1 weight. 
As described in the main text, DII is capable of discovering valuable semantic cues from a large number of weak annotations, thus addressing inconsistency among weakly-annotated instances.

\Fig\ref{fig:polyp_comparison_supp} shows additional qualitative results produced by our label-efficient hybrid-supervised method.
Although our framework is trained with only a few strong annotations, it successfully produces high-quality segmentation results for polyps of various sizes.
In contrast, the results produced by the state-of-the-art comparison algorithms contain severely incomplete or cluttered activations. 
In particular, the performance of compared algorithms is often unreliable for severe polyps.
In addition, we also demonstrate the visualization results on the AS-OCT dataset in \Fig\ref{fig:oct_comparison_supp}. Our hybrid supervised framework consistently produces competitive segmentation results.

\begin{figure*}[t!]
    \centering
    \includegraphics[width=0.93\linewidth]{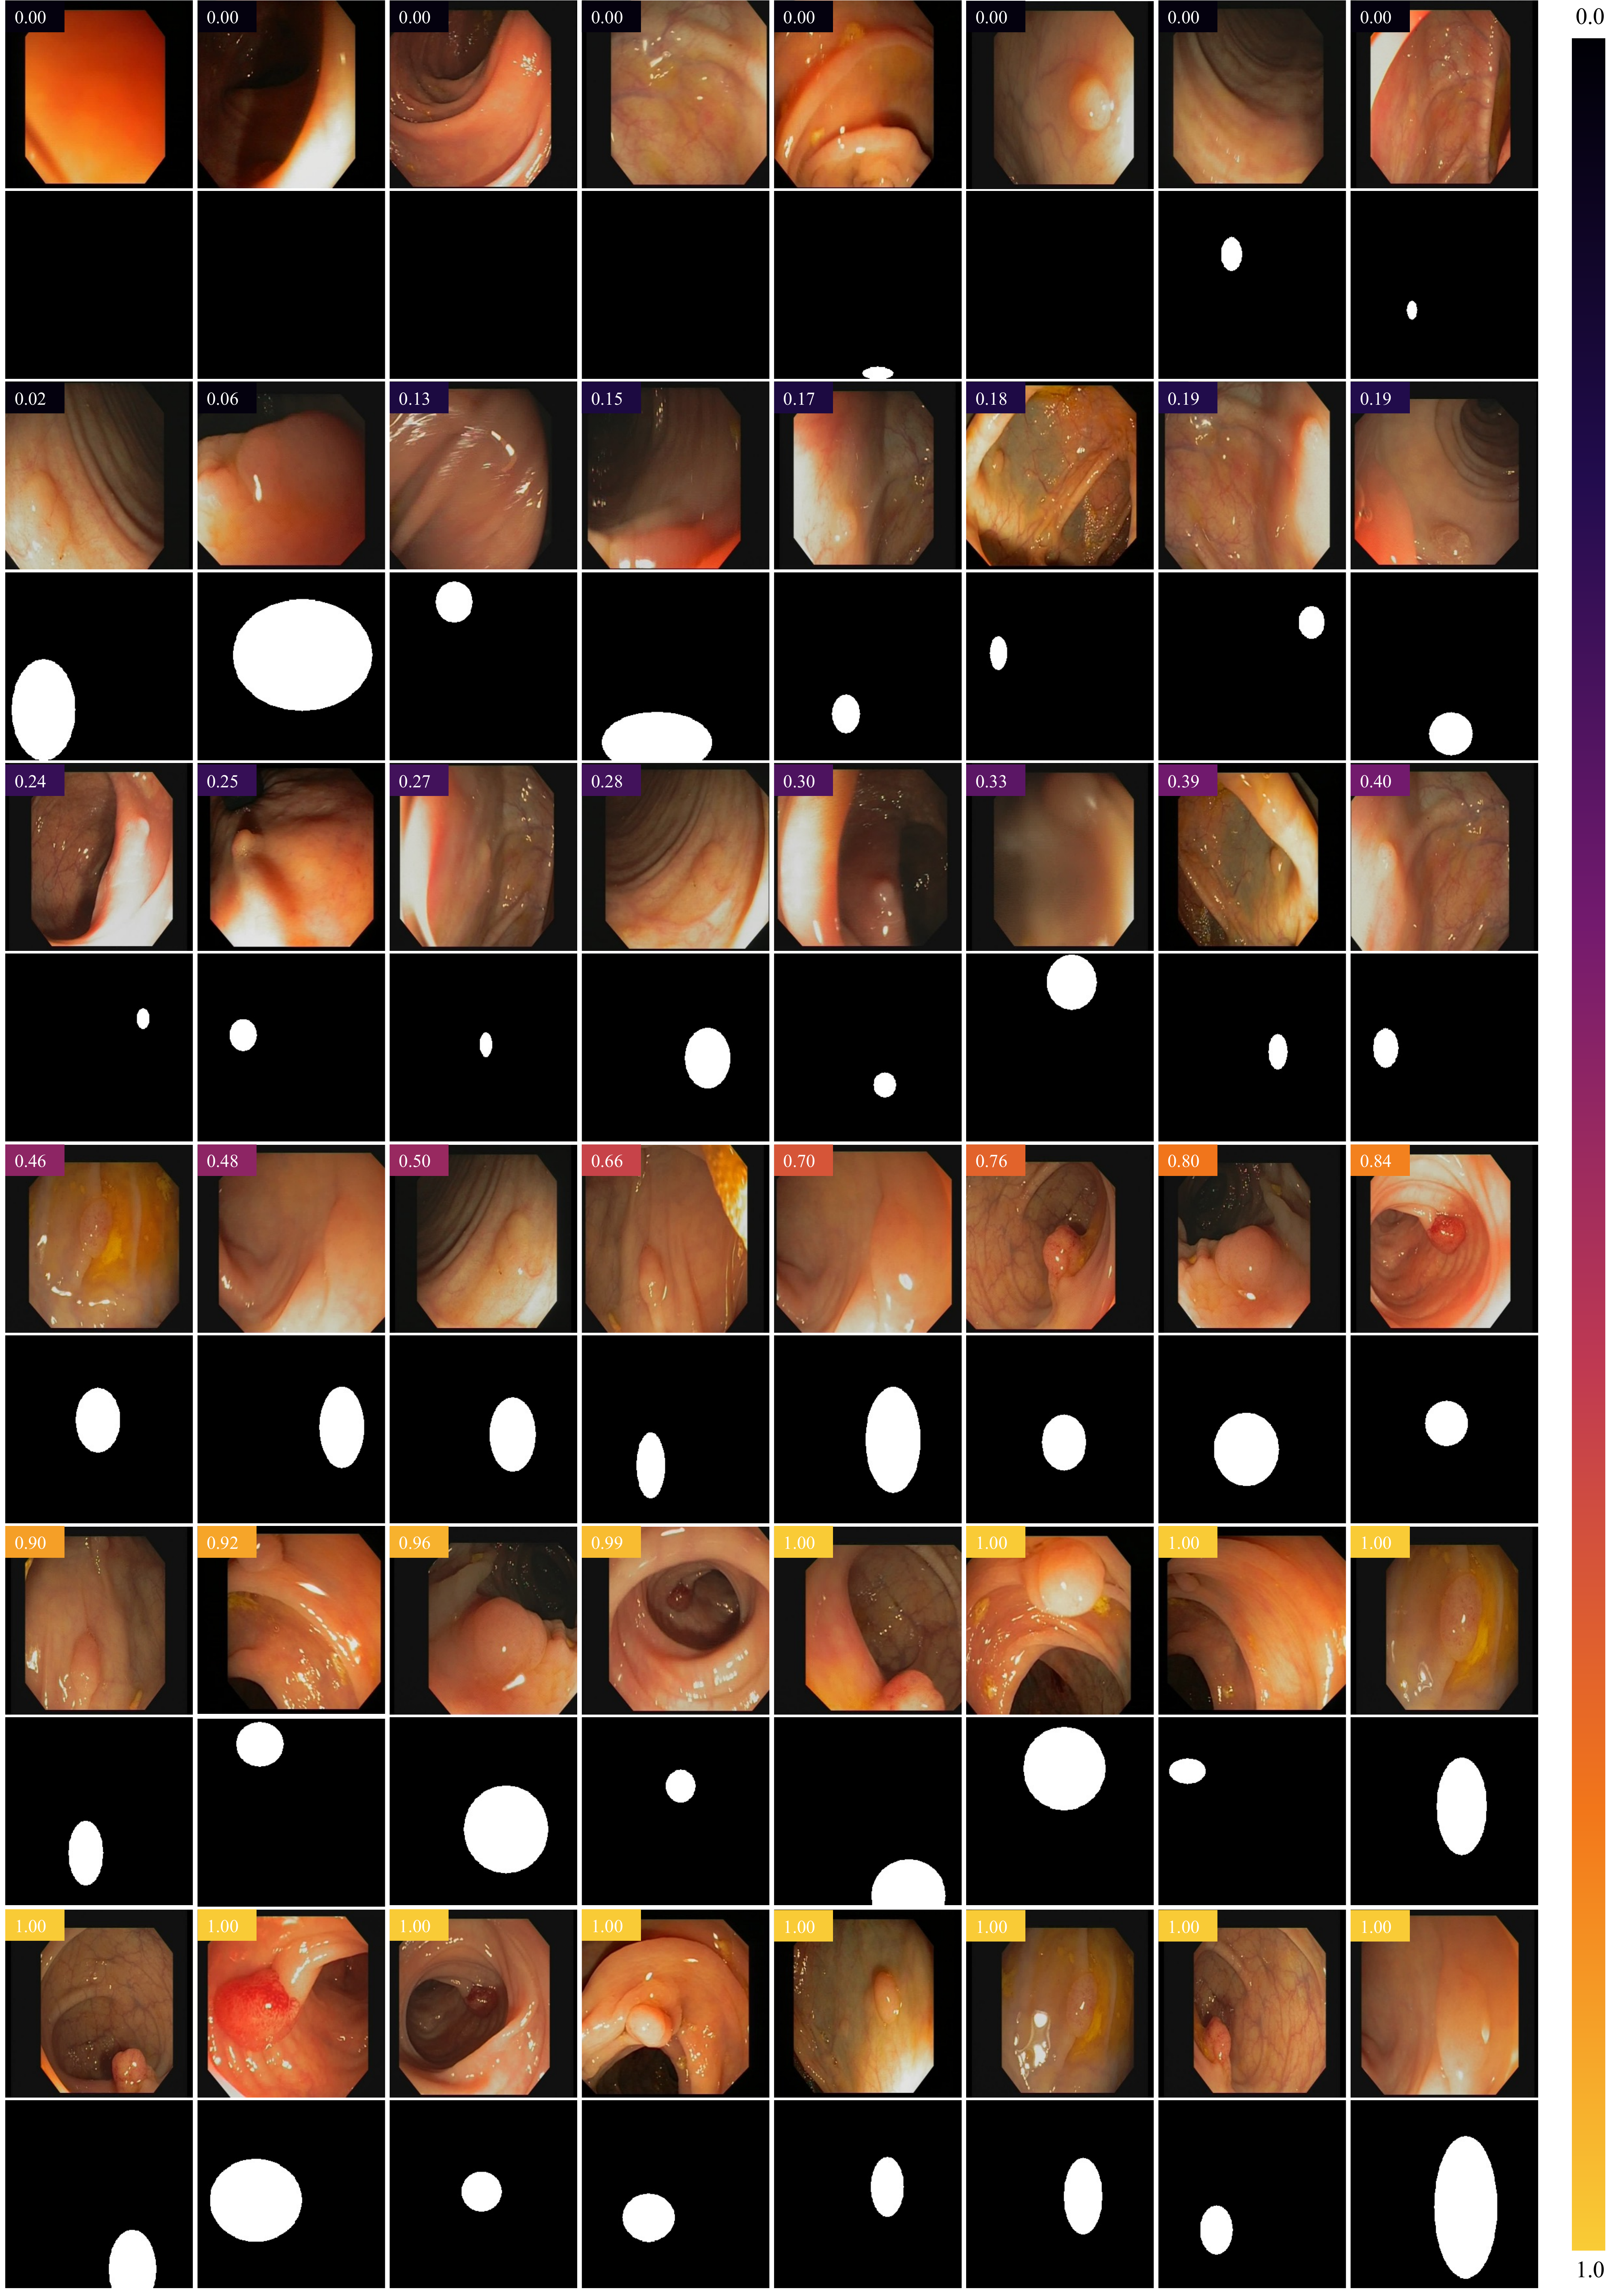}
    \caption{
    Additional demonstrations of DIIs for randomly selected instances. 
    % Here, we illustrate input images, corresponding weak annotations, and DII values.
    }
    \label{fig:dii_supp}
\end{figure*}

\begin{figure*}[t!]
    \centering
    \includegraphics[width=0.95\linewidth]{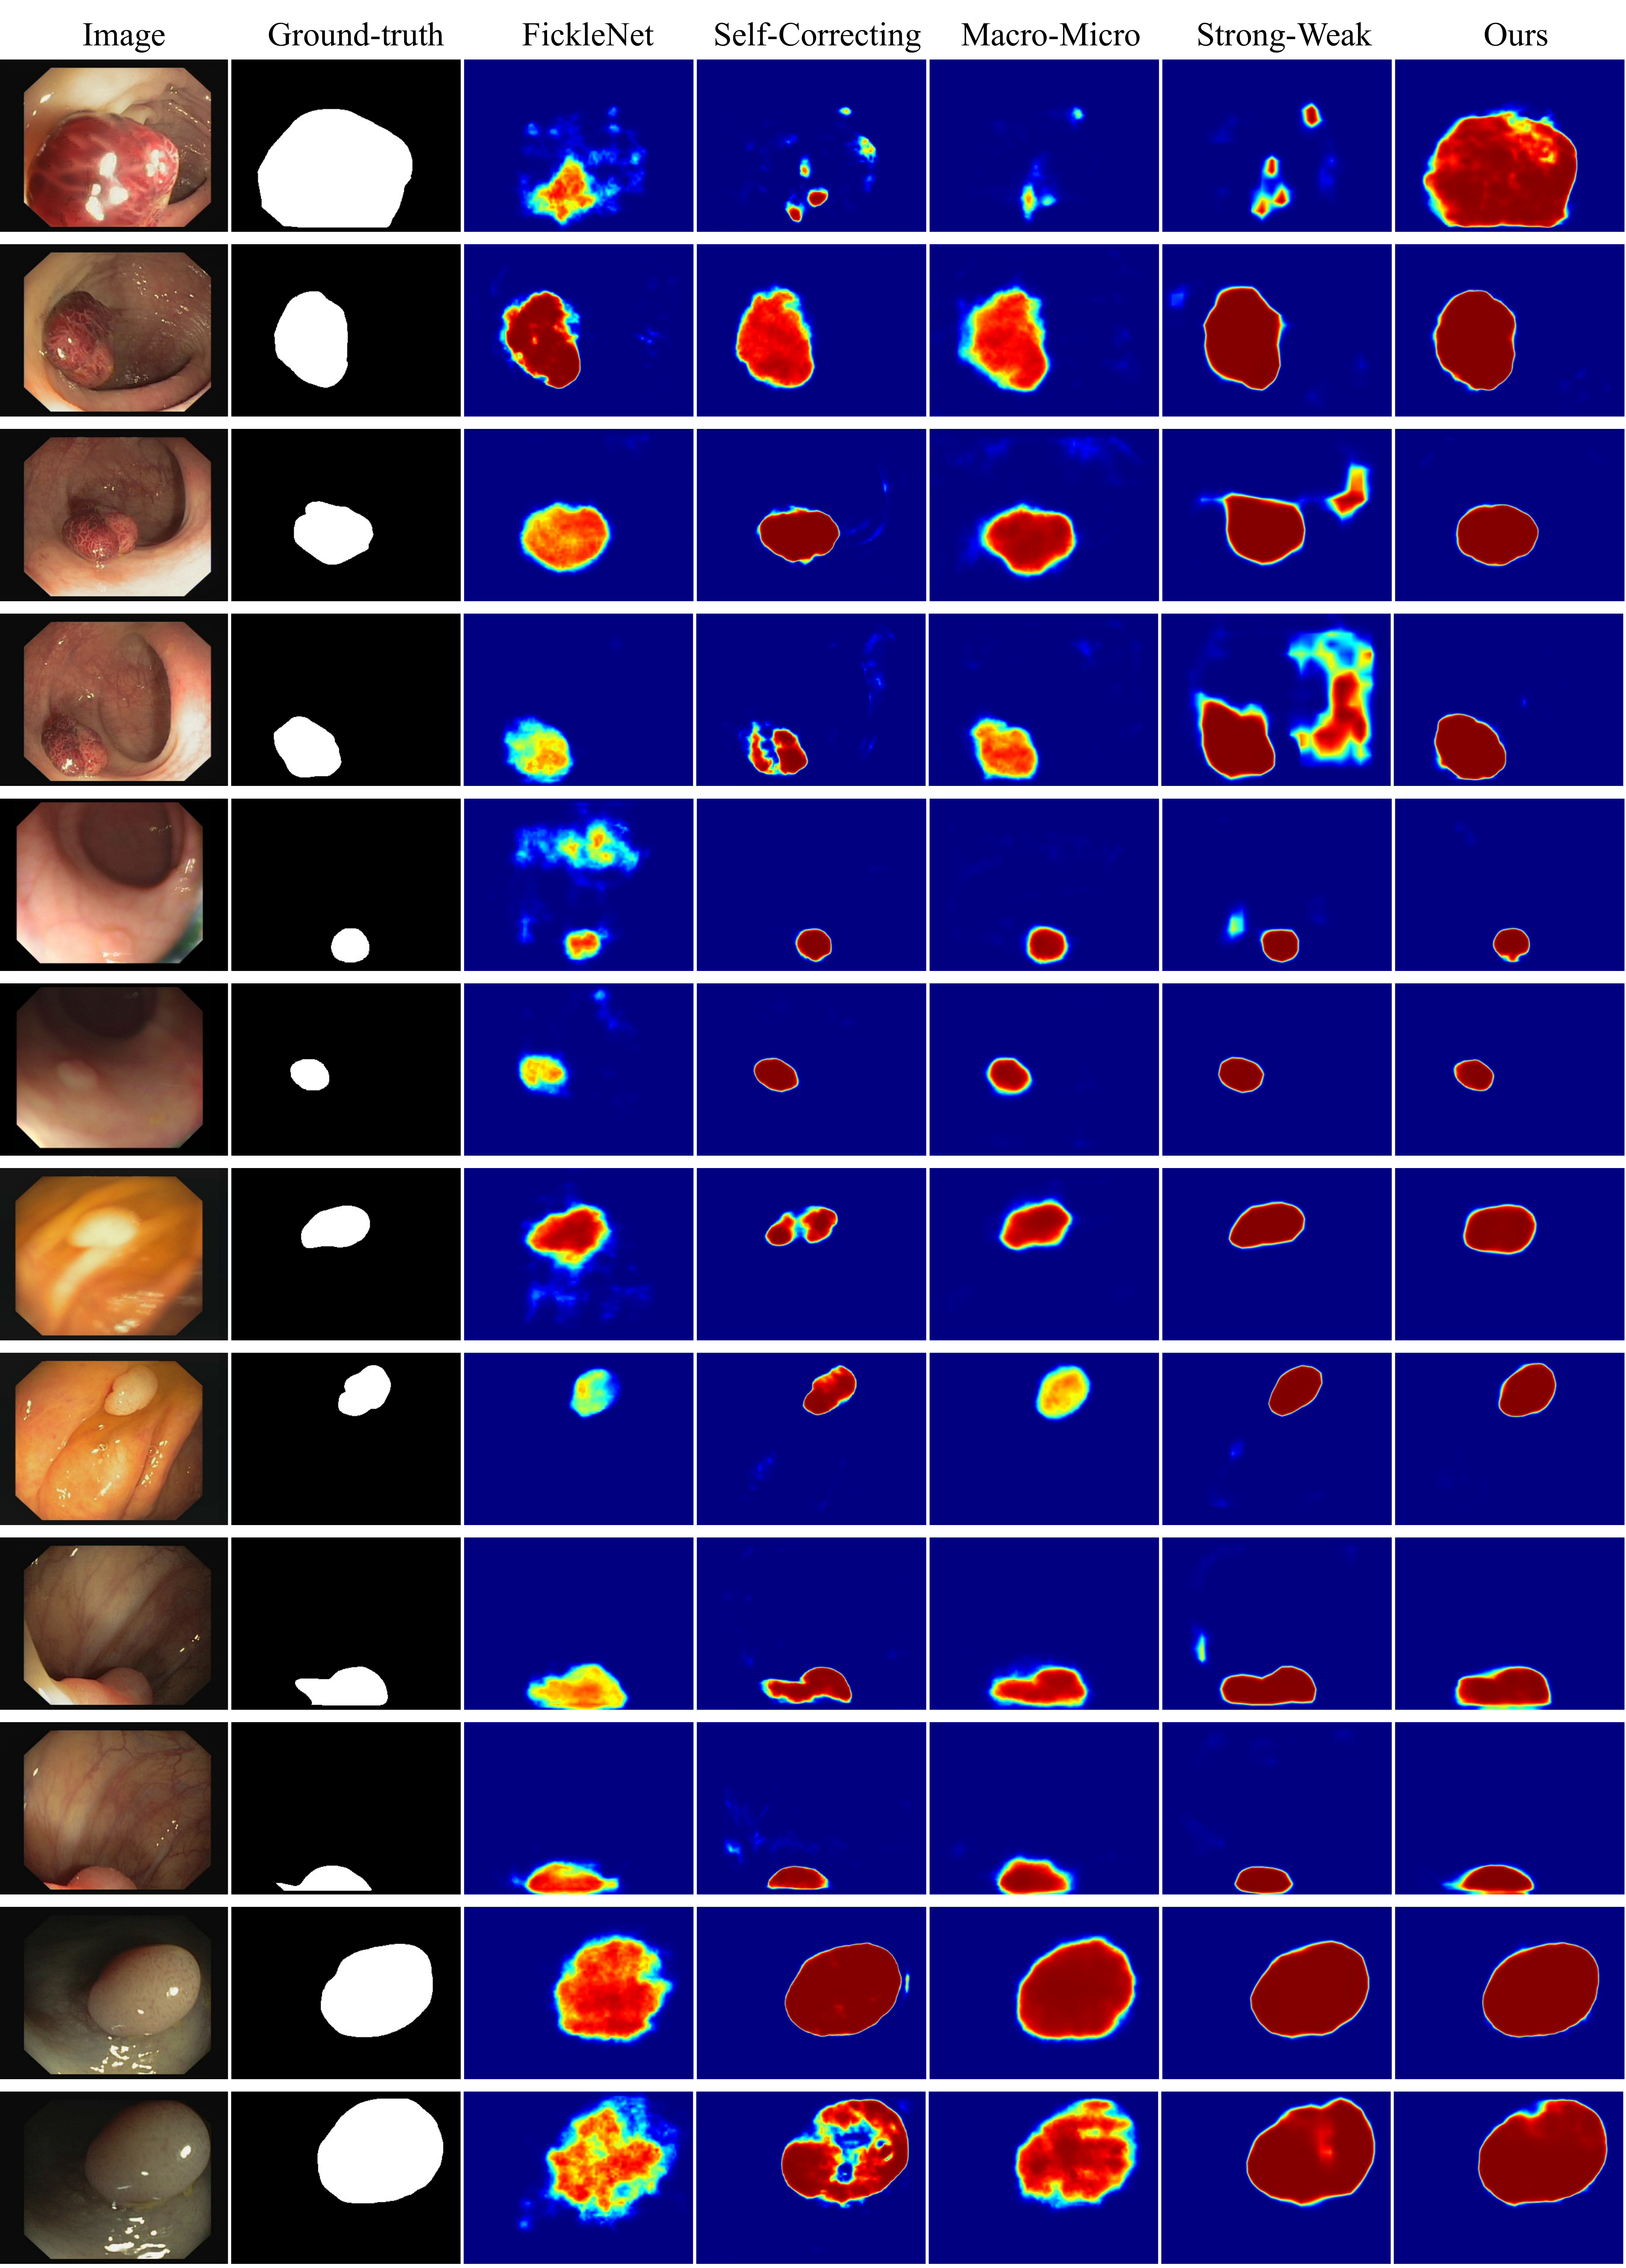}
    \caption{Additional qualitative comparisons of our method with the state-of-the-arts on the polyp segmentation dataset.}
    \label{fig:polyp_comparison_supp}
\end{figure*}

\begin{figure*}[t!]
    \centering
    \includegraphics[width=1.0\linewidth]{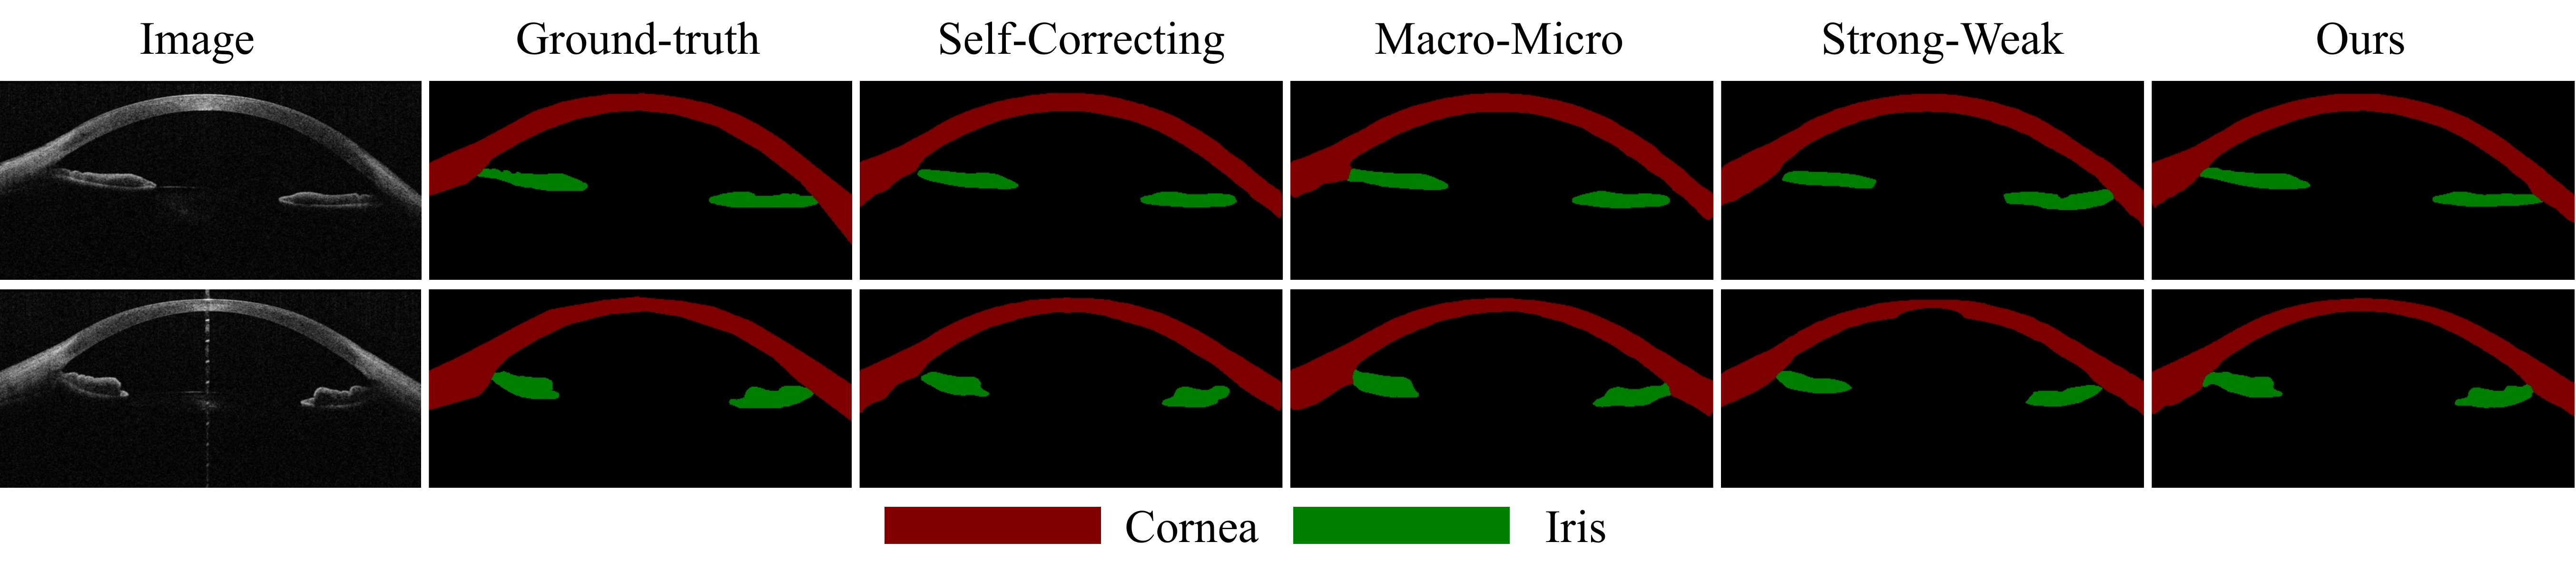}
    \caption{Qualitative comparisons of our method with the state-of-the-arts on the AS-OCT dataset.}
    \label{fig:oct_comparison_supp}
\end{figure*}
